# Supplementary material for: A wireless bilateral transceiver coil based on volume decoupled resonators for a clinical MR mammography
Source: arXiv:2412.20625 source file (2024-12-30)
Supplement: Supplementary file 1 [file Suplementary.tex]

\documentclass[num-refs]{wiley-article}
% : import packages
% : required packages
\usepackage{geometry}  % Flexible and complete interface to document dimensions
\usepackage[section]{placeins}
\usepackage{siunitx}
\usepackage{amsmath}
\usepackage{multirow,multicol}
\usepackage{graphicx}
\usepackage{tabularx}
\usepackage{epstopdf}
\usepackage{hyperref}
\usepackage{dcolumn}
\usepackage{bm}
\usepackage{ulem}
\usepackage[T1]{fontenc}  % Standard package for selecting font encodings
\usepackage{lineno}  % Line numbers on paragraphs
\usepackage{fancyhdr}  % Extensive control of page headers and footers in LaTeX2ε
\usepackage{enumitem}  % Control layout of itemize, enumerate, description
\usepackage{hyperref}  % Extensive support for hypertext in LaTeX
\usepackage{titling}  % Control over the typesetting of the \maketitle command
\usepackage{filecontents}
\usepackage{mathtools}  % Mathematical tools to use with amsmath
\usepackage{titlesec}  % Select alternative section titles
\usepackage{lastpage}  % Reference last page for Page N of M type footers
\usepackage{amsmath}  % AMS mathematical facilities for LaTeX
\usepackage{amsfonts}  % TeX fonts from the American Mathematical Society
\usepackage{amssymb}  % Additional symbols from American Mathematical Society
\usepackage{wasysym}  % LaTeX support file to use the WASY2 fonts
\usepackage{bbm}  % "Blackboard-style" cm fonts
\usepackage{array}  % Extending the array and tabular environments
\usepackage{xr}  % References to other LaTeX documents
\usepackage{verbatim} % Reimplementation of and extensions to LaTeX verbatim
\usepackage{float} % Improved interface for floating objects
\usepackage{marginnote}
\usepackage{todonotes}
\usepackage{ulem}
\AddToHook{cmd/section/before}{\clearpage}
\begin{document}

\section*{Supporting Information\\Quadrature Tx/Rx wireless coil: design concept and application for bilateral breast MRI at 1.5 T}

Viktor Puchnin et al. 
\\
\\
The Supporting Information includes 9 Figures.
\\
\\

\section{Comparison of the unilateral and bilateral designs of the linearly polarized coils}
Previously, we have demonstrated the possibility of improving 
MR visualization of the breast using a unilateral coil based on the metasolenoid, the so-called 
M-coil [35]. However, for clinical diagnostics, 
bilateral design is of greater
interest. The addition of the second M-coil 
leads to a strong coupling between the two resonators, and the initial lowest-frequency resonance splits into two modes: symmetric and antisymmetric (see the spectra in Figure~1B of the main text). In this case,  the initial energy also redistributes between the two resonators, i.e. the field focusing area increases,
while the total absorbed power remains 
the same.  Thus, one can observe a 1.46-fold decrease in the amplitude of the $B_1^+$ (calculated for 1 W of accepted power) in the ROI (Figure~\ref{uni}). As for the $B_1^+$ uniformity (calculated as (1 - deviation of $|B_1^+|_{\rm{ROI}}$/$<B_1^+>$)$\cdot100\%$), it is 91.5\% for the M-coil (calculated over one breast) and 93.6\% for the MM-coil (calculated in both breasts). Moreover, the addition of a second metasolenoid affected the distribution of SAR. The local maximum shifted to the breast area and decreased by 1.8 times. As a result, overall SAR efficiency decreased from 3.08 to 2.84 only. 
\par A similar numerical study was carried out for Helmholtz-type coils. Due to the redistribution of energy between the two resonators, the transmit efficiency for the HH-coil is 1.36 times lower compared to the H-coil. At the same time, the maximum local SAR level is increased by 1.12 times. An increase in local SAR value is a result of a greater concentration of current in the area between the breasts near the skin. The uniformity of the $B_1^+$ field distribution was also estimated. It is 48.4\% for H-coil (calculated over one breast) and 45\% for HH-coil (calculated in both breasts). 

\begin{figure}[htbp]
\renewcommand{\thefigure}{S\arabic{figure}}
\centering
\includegraphics[width=14cm]{B1SUPrev.eps}
\caption{A-D, Schematic view of the numerical setups for a female voxel model placed inside the birdcage coil with the unilateral M-coil (A), bilateral MM-coil (B), unilateral H-coil (C) and bilateral HH-coil (D). E-H, Numerically calculated $|$B$_1^+|_\mathrm{RMS}$ maps for 1 W of total accepted power for the considered setups. The mean $|$B$_1^+|_\mathrm{RMS}$ values were calculated in the breast area. I-L, Numerically calculated SAR$_\mathrm{av.10g}$ maps for 1 W of total accepted power %, shown 
in the plane of the local SAR maximum. The local SAR$_\mathrm{av.10g}$ maxima are indicated with red circles.}
\label{uni}
\end{figure}

\section{Design of the proposed quadrature coil}
\begin{figure}[h!]
\renewcommand{\thefigure}{S\arabic{figure}}
\centering
\includegraphics[width=14cm]{hhmmPCB.eps}
\caption{A. Schematic view of the quadrature HHMM-coil design. Layout of the printed circuit boards (PCBs) for B, MM-coil and C, HH-coil.}

\end{figure}

\begin{figure}[htbp]
\renewcommand{\thefigure}{S\arabic{figure}}
\centering
\includegraphics[width=14cm]{exthhmmPCB.eps}
\caption{A. Schematic view of the extended quadrature HHMM-coil design. Layout of the printed circuit boards (PCBs) for B, MM-coil, and C, HH-coil for the extended HHMM-coil design.}
\end{figure}

\newpage
\section{$\rm{S}_{11}$-parameters of the studied wireless coils}
\begin{figure}[htbp]
\renewcommand{\thefigure}{S\arabic{figure}}
\centering
\includegraphics[width=12cm]{supspar.eps}
\caption{Experimentally measured S$_{11}$-parameters of the loop antenna placed near each pair of the resonators. The position of the antenna is shown by blue lines.}
\end{figure}

\section{Numerically calculated ${\rm{B_1^+}}$ maps for different wireless coils in the axial, sagittal, and coronal planes.}

\begin{figure}[htbp]
\renewcommand{\thefigure}{S\arabic{figure}}
\centering
\includegraphics[width=11cm]{b1supplanes.eps}
\caption{Numerically calculated $|$B$_1^+|_\mathrm{RMS}$ maps for 1 W of total accepted power for the HH-coil (A-C), MM-coil (D-F), HHMM-coil (G-I) and extended HHMM-coil (J-L) in the axial, sagittal and coronal planes.}
\end{figure}

\section{Electric field distribution of the studied wireless coils}
\begin{figure}[htbp]
\renewcommand{\thefigure}{S\arabic{figure}}
\centering
\includegraphics[width=12cm]{efields2.eps}
\caption{Schematic view of linear and quadrature coils' designs: A, a pair of Helmholtz-type coils (the HH-coil); B, a pair of `metasolenoid'-based coils (the MM-coil);  C, a quadrature coil based on the combination of linearly polarized coils (the
HHMM-coil). Numerically calculated E-field maps for 1 W of total accepted power in the axial (D-F) and sagittal (G-I) planes.}
\end{figure}

\section{Local minimum of the magnetic field in the body connected with using MM-coil}
\par MR images obtained with the extended HHMM coil have a tiny local minimum between two breasts in the chest wall in the axial plane (Figure 6 of the main text). The reason, for its appearance, is the interaction between two y-polarized MM-coils. The currents on the neighboring tubes of the lower rings of the MM-coil flow in the opposite phase. In other words, when the proposed resonators interact, the magnetic field B1 in the center of the breast wall begins to rotate in the opposite direction, compared to the field in the breast (see Figure~\ref{minimum}). This can be corrected by using a large metasolenoid instead of two small ones, however, this will reduce the transmit efficiency. In the meanwhile, this local minimum does not affect significantly the diagnostic accuracy of the image.

\begin{figure}[h!]
\renewcommand{\thefigure}{S\arabic{figure}}
\centering
\includegraphics[width=12cm]{minimumrev.eps}
\caption{A-B, Schematic view of the numerical setups for a female voxel model placed inside the birdcage coil with the MM-coil (A) and the HHMM-coil (B). C-D, Numerically calculated $|$B$_1^+|_\mathrm{RMS}$ maps for 1 W of total accepted power for the considered setups. E-F, Numerically calculated vector distribution of $B_1^+$ in the region of the local minimum.}
\label{minimum}
\end{figure}

\section{Transmit efficiency enhancement using linear and quadrature metamaterial-inspired wireless coils}

\par The proposed quadrature HHMM-coil provides more than 2 times greater gain in transmit efficiency compared to the linearly polarized MM-coil that is higher than expected gain of a $\sqrt{2}$. A larger than expected gain could be explained by the suboptimal excitation of a linearly polarized MM-coil using a quadrature birdcage coil. In this case, the MM-coil interacts only with the $H_y$-component of the magnetic field. Thus, part of the power supplied to the birdcage coil does not contribute to the MM-coil excitation. In order to demonstrate this, we conducted a numerical simulation that included a y-polarized birdcage coil with a voxel model and the MM-coil. The results are presented in Figure~\ref{amp}. In the case of the linearly polarized birdcage coil, the amplitude of the RF magnetic field in the breast tissues became 1.7 times larger relative to the case of MM-coil excitation using the quadrature birdcage. Also, the $B_1^+$ field amplitude of the quadrature HHMM-coil with quadrature excitation is 1.32 times higher than for the linear MM-coil with linear excitation. This value is slightly less than the $\sqrt{2}$, which is typical for the classical case. Thus, the more than 2 times transmit efficiency gain demonstrated in the work is connected with the fact that the linearly polarized wireless coil works suboptimally in a quadrature birdcage coil and can be much more effective with the linear excitation (for example, in MR scanners with saddle-coil).

\begin{figure}[htbp]
\renewcommand{\thefigure}{S\arabic{figure}}
\centering
\includegraphics[width=12cm]{ampl.eps}
\caption{Numerically calculated $|$B$_1^+|_\mathrm{RMS}$ maps for 1 W of total accepted power for the linear-polarized (A) and quadrature (B) birdcage coil without any resonator and in combination with the MM-coil (C,D) or the HHMM-coil (E).}
\label{amp}
\end{figure}

\section{Investigation of the possibility of using the HHMM-coil in the birdcage coil with different bore diameters}

In order to demonstrate the HHMM-coil operation in different geometries of the birdcage coils, we carried out numerical studies using birdcage coils with different bore diameters of 70 cm and 60 cm. Initially, the extended quadrature coil was adjusted to be used in a 70 cm bore diameter. It has the following parameters: the M-coil tubes' length was 152 mm, and the capacitance value of variable capacitors of the H-coil was equal to 9.5 pF. More details can be found in the main text (Methods) and in Supporting Information (Section “Design of the proposed quadrature coil”). In this case, the coil provides a transmit efficiency of 2.1 $\rm{\mu T}/\sqrt{P}$ (Figure~\ref{bore60}A). However, the placement of the same coil in a 60-cm bore leads to quadrature coil detuning from its original symmetric hybrid mode, thus its efficiency decreases to a value of 0.7 $\rm{\mu T}/\sqrt{P}$ for the same ROI (Figure~\ref{bore60}B). However, after fine-tuning both types of resonators (MM- and HH-coils) one can obtain the $B_1^+$ field distribution similar to the model with a 70 cm diameter (Figure~\ref{bore60}C). In this case, the length of the telescopic tubes was 150 mm, while the capacitance in H-coil was changed to 8.7 pF. In the experimental studies, the tuning was carried out by changing the capacitance of the variable capacitors of the Helmholtz-type coils and changing the length of the telescopic tubes of the metasolenoids.

\begin{figure}[htbp]
\renewcommand{\thefigure}{S\arabic{figure}}
\centering
\includegraphics[width=14cm]{hhmm7060.eps}
\caption{Numerically calculated $|$B$_1^+|_\mathrm{RMS}$ maps for 1 W of total accepted power for the HHMM-coil placed inside a birdcage coil with 70 cm (A) and 60 cm (B, C) bore diameter. The HHMM-coil configuration was the same in panels A-B, and changed (tuned) in panel C.}
\label{bore60}
\end{figure}

\end{document}
